# Supplementary material for: Magnetochiral Properties of Spin Waves Existing in Nanotubes with Axial and Circumferential Magnetization
Source: arXiv:2204.12995 ancillary file (2022-04-27)
Supplement: Supplementary file 1 [file BLS_Magnetochiral_SpinWaves_Tubes_SI.pdf]

# Supplemental Material of "Magnetochiral Properties of Spin Waves Existing in Nanotubes with Axial and Circumferential Magnetization"

M.C. Giordano, M. Hamdi, and A. Mucchietto
*École Polytechnique Fédérale de Lausanne, School of Engineering, Institute of Materials, Laboratory of Nanoscale Magnetic Materials and Magnonics, 1015 Lausanne, Switzerland*

D. Grundler*
*École Polytechnique Fédérale de Lausanne, School of Engineering, Institute of Materials, Laboratory of Nanoscale Magnetic Materials and Magnonics, 1015 Lausanne, Switzerland and École Polytechnique Fédérale de Lausanne, School of Engineering, Institute of Electrical and Micro Engineering, 1015 Lausanne, Switzerland*

(Dated: April 26, 2022)

## I. METHODS

### A. Samples fabrication

Nanotubes were fabricated by coating, via a plasma enhanced atomic layer deposition (PE-ALD) process, the ferromagnetic permalloy $Ni_{80}Fe_{20}$ (Py) onto GaAs nanowires (NWs) previously grown on Si (111) substrates in a moelcular-beam epitaxy reactor as reported in Ref. S1. The PE-ALD process was performed in a hot wall Beneq TFS 200 ALD reactor as described in Ref. S2. The largest external diameter of the nanotube hexagon was measured by SEM micrography, assuming that the NT was lying on one of the hexagon facets. The internal diameter was estimated by subtracting twice the average thickness of the ferromagnetic coating, measured with TEM microscopy. The Py NTs were transferred trough an isopropyl alcohol solution on a 4-inch Si(100) wafer covered with 200 nm thick $SiO_2$ with pre-patterned gold alignment markers for the fabrication of integrated coplanar waveguides (CPWs). The metallic CPWs were prepared by electron beam lithography and a following evaporation of 5 nm Ti/ 120 nm Au film. The CPWs' dimensions were chosen to enable impedance matching. The signal line, having a width of $2.6 \pm 0.1$ $\mu$m was separated by gaps of $1.7 \pm 0.1$ $\mu$m width from the the ground lines. The CPW was fabricated in a way that the signal line was parallel to the long axis of the NT, placed in one of the gaps.

### B. Spin waves excitation-detection scheme

Spin wave eigenmodes were detected via microfocus Brillouin light scattering ($\mu$-BLS) microscopy at room temperature [S3, S4]. The CPW was electrically connected via wire bonding and a printed circuit board to a signal generator (Anritsu MG3692C) applying current. The corresponding magnetic microwave field excited spin precession in the NT at a fixed frequency. The frequency was varied in a step-wise manner from 2.5 to 12.5 GHz. A monochromatic laser with a wavelength of 473 nm and power of 0.5 mW was focused on the top surface of the NT. The recorded BLS signal was proportional to the square of the amplitude of the dynamic magnetization at the position of the laser spot. The sample was mounted on a closed loop piezo-electrical stage which allowed a precise positioning of the NT. The power was such that spin precession was excited in the linear regime. A magnetic field was applied parallel to the NT long axis (**z** axis) via a permanent magnet mounted on a translation stage. The magnitude of the magnetic field is adjusted by changing the distance between magnets and sample. For the experiment on the sample NT-s1 (NT-s2) the static field was swept from +90 mT to +10 mT in steps of 4 mT (8 mT), from +7 mT to -7 mT in steps of 7 mT and again from -10 mT to -90 mT in steps of 4 mT (8 mT).The field of |7| mT corresponds to the minimum distance of the permanent magnet. Zero field has been reached by removing the permanent magnet.

---

* dirk.grundler@epfl.ch

### C. Micromagnetic simulations

Micromagnetic simulations using OOMMF [S5] were performed to obtain a microscopic insight into SW excitations in NTs. A bitmap containing the required hexagonal geometry of the NT cross section in xy-plane was imported into OOMMF. This hexagonal cross section was rotated along z-axis by 15 degree in order to distribute the systematic roughness due to pixelization on all facets of NTs as uniform as possible (see Figure S1).

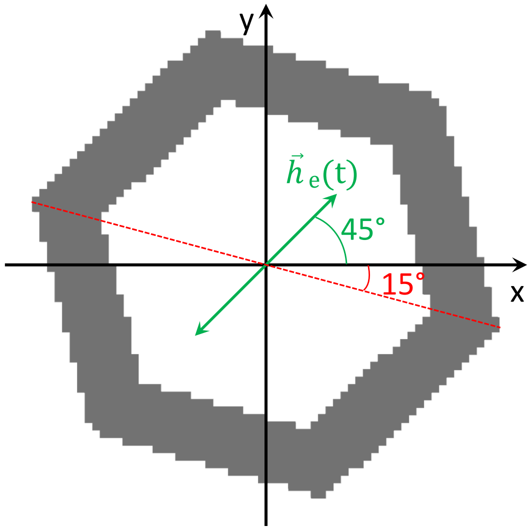


FIG. S1. NT cross section set as input for the micromagnetics simulations. The two ends of the NT are tilted at an angle of 15° with respect to xy-plane to emulate the irregular orientation of the defects in the measured NT. A spatially uniform sinc pulse $\boldsymbol{h_e}$ is applied at 45° with respect to xy-plane. The geometry is discretized on a grid of 2.5 nm × 2.5 nm× 5 nm.

This cross section was extended to L = 560 nm as the length of the simulated NTs. The two ends of the NT is terminated at an angle of 15 degree with respect to xy-plane to emulate the irregular orientation of the defects in the measured NT. The geometry is discretized on a grid of 2.5 nm×2.5 nm×5 nm. A uniform DC magnetic field was applied along the z direction (NT axis), and equilibrium magnetization configuration was determined for each DC field value. Subsequently, a spatially uniform Sinc pulse of the form

$$\boldsymbol{h_e} = h_0 \left( \frac{\sin\left(2\pi f_c (t - t_0)\right)}{2\pi f_c (t - t_0)} \right) \left[\cos(45^\circ)\ \hat{x} + \sin(45^\circ)\ \hat{y}\right] \tag{S1}$$

with amplitude of $h_0 = 2$ mT, cut-off frequency of $f_c = 50$ GHz and $t_0 = 500$ ps was applied at an angle of 45° in the xy-plane. A total simulation duration of T = 5 ns was considered. The dynamic magnetization was recorded as a function of x, y, z every time step of $\delta$t = 5 ps. A fast Fourier transformation (FFT) was performed on the magnetization of each pixel along the time axis to obtain the resonance spectrum. Then sums of power and phase of complex dynamic magnetization $m_d = m_x + im_y$ were calculated to display the SW spatial profile for relevant frequencies. $\mid m_d \mid$ was then integrated over the whole geometry (defined as PSD), and plotted as a function of frequency $f$ in order to observe the microwave absorption. The input parameters used in the simulations were as follows: saturation magnetization $M_s$ = 800 kA/m, exchange constant A = 13 pJ/m, and damping constant $\alpha$ = 0.005. The dynamic magnetization profiles are visualized using "Mayavi: 3D Visualization of Scientific Data" [S6].

## II. SUPPLEMENTARY RESULTS

### A. BLS measurement on a second sample

The same BLS experiment has been performed on two individual Py NTs with the same scheme based on microwave excitation via a CPW antenna and $\mu$-BLS laser spin waves detection. Figure S2 shows the micrographs of the two samples. In Figure S3 the BLS spectra measured on the sample NT-s2 are reported as a function of the external applied field.

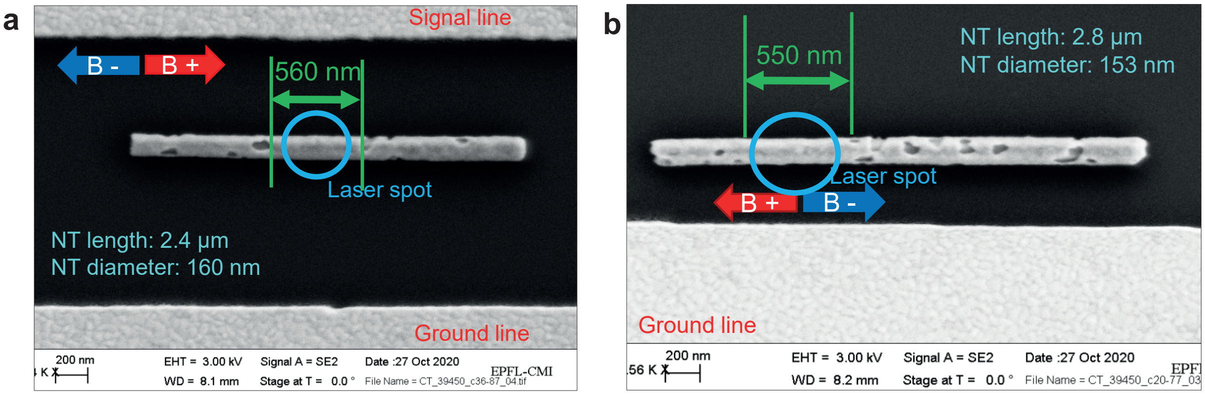


FIG. S2. SEM micrographs of (a)NT-s1 and (b) NT-s2. The relevant geometrical parameters are indicated on the picture and are summarized in Table II A. The BLS laser position and its diameter is approximately given by the blue circles depicted. Positive and negative direction of the external applied fields are depicted, respectively, with red and blue arrows.

TABLE S1. Geometrical parameters of the Py NTs investigated.

| Sample name | Py shell thickness (nm) | External diameter $D_{out}$ (nm) | NT full length $l$ ($\mu$m) | Distance between defects L (nm) |
|---|---|---|---|---|
| NT-s1 (main text) | 22 ± 1 | 160 ± 10 | 2.4 ± 0.1 | 560 ± 10 |
| NT-s2 | 22 ± 1 | 153 ± 10 | 2.8 ± 0.1 | 550 ± 10 |

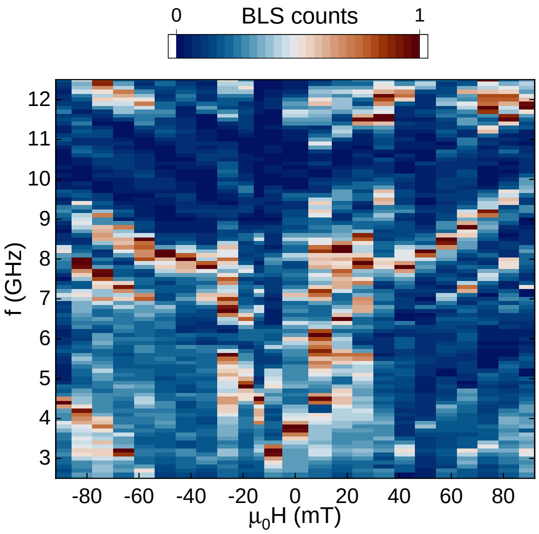


FIG. S3. BLS spectra detected at room temperature at the center of the sample NT-s2, plotted as a function of an external static magnetic field $\mu_0 H$ applied along the NT axis.

## B. Static micromagnetic simulations

In Figure S4 we report the results of the simulated static magnetization of a Py NT initially magnetized along its axis (**z** direction). The figure shows the magnetic hysteresis obtained by extracting the magnetization along **z** ($M_z$) as a function of the static magnetic field $\mu_0 H_z$ along the same direction. The field was swept from positive to negative values (red curve) and from negative to positive values (blue curve). Depictions of the simulated NT magnetization are given at specific values of magnetic field selected on the red curve. For high positive magnetic fields $\mu_0 H_z > 33$ mT a magnetic state approximated by a saturated state is found, where most of the spins are alligned along **z**. The spin configuration is depicted for an applied field of 76 mT. Moving from high positive magnetic field towards zero, we

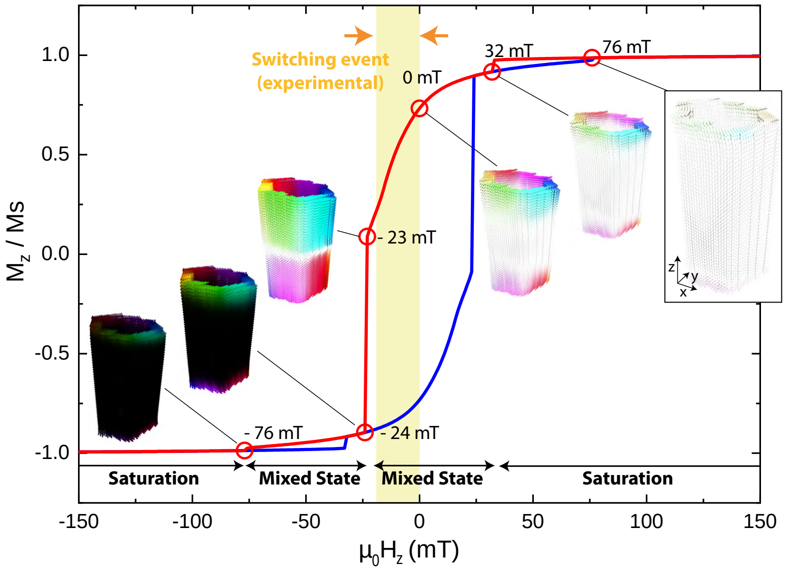


FIG. S4. Simulated static magnetization hysteresis of a Py NT magnetized along its axis (**z** direction) when the field is swept from positive to negative values (red curve) and from negative to positive values (blue curve). Magnetic configurations are extracted from the simulations at specific fields and displayed for +76, + 32, 0, -23, -24 and -76 mT.

observe that the relative magnetization stays at almost 1 until +33 mT and then drops to a value of 0.9 at +32 mT. At 32 mT the magnetization curls at the ends of the tube to minimize the stray field and remains axially in the center to minimize the exchange energy. The end-vortices show opposite chirality as expected for thick tubes with $t/r_0 > 0.2$ [S7]. This magnetic configuration is known as the mixed state. With $\mu_0 H_z$ decreasing from 32 mT to 0 mT, $M_z/M_s$ is found to decrease monotonously down to 0.7. At $\mu_0 H_z$= 0 the ground state is still the mixed state. The relative magnetization reduces to zero for a magnetic field value of -23 mT. Here, the end-vortices having opposite senses of rotations, have expanded such that they are separated by a Néel-type domain wall located in the center. At -24 mT a switching event occurs whereby the central magnetization changes sign, leading to the formation of a mixed state with magnetization aligned along the negative **z** axis in the central part of the nanotube approaching $M_z/M_s$ = -0.9. The formation of the saturated magnetic state is observed starting from -76 mT. The magnetic field range where the BLS data suggest a decrease of relative NT magnetization terminating in a switching event (from 0 to - 18 mT) is highlighted in yellow for comparison with the simulated hysteresis.

### C. Dynamic micromagnetic simulations

In Figure S5, we report the power spectral density (PSD), outcome of the dynamic micromagnetic simulations, as a function of an external applied field. The spectra shown in the main text of the manuscript are extracted from this 2D map at specific fields (+ 58 mT, 0 mT, -14 mT).

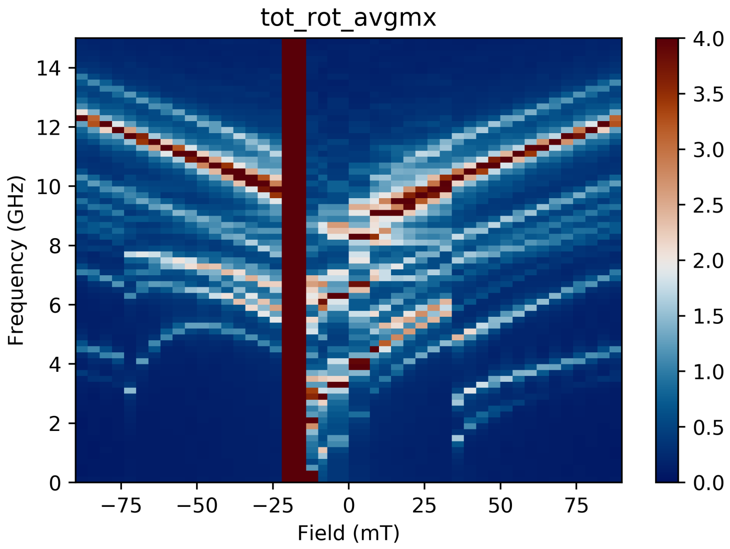


FIG. S5. Power spectral density (PSD), outcome of the dynamic micromagnetic simulations, as a function of an external applied field.

First two authors M. C. Giordano and M. Hamdi contributed equally to this work.

[S1] F. Matteini, G. Tütüncüoglu, D. Mikulik, J. Vukajlovic-Plestina, H. Potts, J.-B. Leran, W. C. Carter, and A. Fontcuberta i Morral, Impact of the ga droplet wetting, morphology, and pinholes on the orientation of gaas nanowires, Crystal Growth & Design **16**, 5781 (2016).

[S2] M. C. Giordano, S. Escobar Steinvall, S. Watanabe, A. Fontcuberta i Morral, and D. Grundler, $Ni_{80}fe_{20}$ nanotubes with optimized spintronic functionalities prepared by atomic layer deposition, (2021), arXiv2105.01969.

[S3] V. E. Demokritov, S. O. & Demidov, Micro-brillouin light scattering spectroscopy of magnetic nanostructures, IEEE Trans. Magn. **44**, 6–12 (2008).

[S4] T. Sebastian, K. Schultheiss, B. Obry, B. Hillebrands, and H. Schultheiss, Micro-focused Brillouin light scattering: imaging spin waves at the nanoscale, Frontiers in Physics **3**, 35 (2015).

[S5] M. J. Donahue and D. G. Porter, *OOMMF user's guide, version 1.0* (US Department of Commerce, National Institute of Standards and Technology, 1999).

[S6] P. Ramachandran and G. Varoquaux, Mayavi: 3D visualization of scientific data, Computing in Science & Engineering **13**, 40 (2011).

[S7] A. P. Chen, J. M. Gonzalez, and K. Y. Guslienko, Magnetization configurations and reversal of magnetic nanotubes with opposite chiralities of the end domains, Journal of Applied Physics **109**, 073923 (2011).
